# Supplementary material for: Hybrid SLC-MLC RRAM Mixed-Signal Processing-in-Memory Architecture for Transformer Acceleration via Gradient Redistribution
Source: arXiv:2506.00020 source file (2025-05-20)
Supplement: Supplementary file 1 [file appendix.tex]

\section*{Appendix}

\subsection*{A. Abstract}
This section describes the process to reproduce the key experimental results of the BERT-Base, BERT-Large, and Llama3 models shown in Figure~12, focusing on inference performance degradation under analog noise in a hybrid RRAM-based processing-in-memory (PIM) accelerator. Our simulator emulates the analog non-idealities by injecting noise into the weight matrices and measures the inference loss to evaluate the effectiveness of single-level cell (SLC) mapping based on gradient importance. The full workflow includes: (1) model and dataset preparation, (2) pre-SVD fine-tuning (optional), (3) low-rank decomposition using singular value decomposition (SVD) for linear layers and post-SVD truncation, (4) fine-tuning with gradient redistribution, and (5) noise-injected inference to evaluate the accuracy or loss.

\subsection*{B. Artifact Check-list}
\begin{itemize}
  \item \textbf{Program}: HyFlexPIM noise-aware simulator (this repository).
  \item \textbf{Compilation}: Not required (Python-based Jupyter Notebook).
  \item \textbf{Model \& Dataset}: meta-llama/Llama-3.2-1B (Llama3) with PTB dataset (default) and bert-large-uncased (bert-base-uncased) with GLUE dataset, user-customizable.
  \item \textbf{Run-time environment}: Python 3.8.2+, Jupyter Notebook. Linux (e.g., Ubuntu 20.04+) is recommended for GPU training.
  \item \textbf{Hardware}: Used NVIDIA RTX A6000 GPU with 48GB VRAM (used for fine-tuning).
  \item \textbf{Metrics}: Inference accuracy or loss under different device noise levels and the proportion of weights mapped to SLC.
  \item \textbf{Output}: Accuracy or loss \& perplexity.
  \item \textbf{Disk space required}: Approximately 30~GB (for model checkpoints and gradients).
  \item \textbf{Total experiment time}: Approximately 2--4 hours (depending on fine-tuning).
  \item \textbf{Publicly available}: Yes.
  \item \textbf{License}: MIT License.
  \item \textbf{DOI}: \texttt{10.5281/zenodo.15103949}.
\end{itemize}

\subsection*{C. Description}

\textbf{1) How to access:} \\
All source code, notebook, and utility files are available at: \\
\url{https://github.com/songchangeun96/HyFlexPIM} 

\noindent \textbf{2) Hardware dependencies:} \\
We recommend using a GPU with at least 48~GB of memory for training steps. Our experiments were conducted using two NVIDIA RTX A6000 GPUs (48~GB each). No custom hardware is required.

\noindent \textbf{3) Software dependencies:} \\
Python 3.8.2+, with packages listed in \texttt{requirements.txt}. The simulation runs via Jupyter Notebook and uses PyTorch as its core ML framework.

\subsection*{D. Installation}

\vspace{-0.5em}
\begin{verbatim}
$ git clone 
  https://github.com/songchangeun96/HyFlexPIM.git
$ cd HyFlexPIM
$ pip install -r requirements.txt
$ jupyter notebook HyFlexPIM_llama3.ipynb 
 (or jupyter notebook HyFlexPIM_BERT.ipynb)
\end{verbatim}

\subsection*{E. Experiment Workflow}
The following steps reproduce the result of Llama3 in Figure~12 (Same steps are applied to the BERT model):

\begin{enumerate}[label=\textbf{Step \arabic*:}, leftmargin=3em, rightmargin=2em]
  \item Load the default LLaMA-3.2 1B model and PTB dataset (BERT-Large or BERT-Base model and GLUE dataset for BERT implementation). Optionally, evaluate with \texttt{evaluate\_model()}. Users may also substitute the default model with a quantized custom model of their choice.
  
  \item Fine-tune for 2--3 epochs to improve noise robustness, then merge weights using \texttt{model.merge\_and\_unload()} to apply all fine-tuned parameters to the base model before noise injection.
  
  \item Apply SVD to linear layers and truncate by using \\ \texttt{replace\_linear\_layer\_llama()}.
  
  \item Fine-tune the model and save gradient of $\Sigma$ to \texttt{./gradient/}.
  
  \item Reload gradients and inject noise using \\ \texttt{apply\_noise\_to\_llama(model, std, th)}, and evaluate loss.
\end{enumerate}

\subsection*{F. Evaluation and Expected Results}
This simulator measures inference loss (accuracy) under analog noise perturbations for the Llama3 (BERT) models. Initially, applying SVD followed by truncation introduces significant loss (accuracy degradation) due to the reduced rank approximation. Subsequent fine-tuning for a few epochs helps recover performance, resulting in only a modest (approximately 0.2--0.3) increase in loss (less than 1\% of accuracy degradation for BERT) compared to the original pre-truncation model.

After fine-tuning, our noise-injection simulator allows users to evaluate model robustness under varying levels of analog memory noise and SLC configurations. By default, it simulates RRAM-based memory behavior with a noise standard deviation of $\texttt{std} = 0.025$. Additionally, users can adjust the threshold parameter $\texttt{th}$ to specify the desired proportion of weights stored in SLC. Analog noise is then selectively injected only into the remaining weights mapped to low-precision MLC. While the simulator is currently tailored to the BERT summarization and Llama3 generative model, we plan to extend the support of the \texttt{replace\_linear\_layer} function to a broader range of models by improving compatibility in future updates.

%corresponds to roughly a 2\% magnitude-wise error rate. 

%The simulator then reports how the loss evolves under varying noise magnitudes and SLC configurations. 
